# Supplementary material for: MAiVAR: Multimodal Audio-Image and Video Action Recognizer
Source: arXiv:2209.04780 source file (2022-09-11)
Supplement: Supplementary file 1 [file appendix.tex]

% ...

\section{First appendix section}
